# Supplementary material for: Simulation-based Bayesian predictive probability of success for interim monitoring of clinical trials with competing event data: two case studies
Source: arXiv:2412.15899 source file (2024-12-20)
Supplement: Supplementary file 1 [file supp_separate.tex]

\documentclass[AMA,Times1COL]{template_ARXIV2}

\begin{document}
\input{appendix.tex}

\end{document}
